# Supplementary material for: Structural phase stability, electronic structure, magnetic properties and chemical bonding analysis of transition metal ammine borohydrides with amphoteric hydrogen for hydrogen storage
Source: arXiv:2104.08140 source file (2021-04-16)
Supplement: Supplementary file 1 [file supporting_information.pdf]

**Structural phase stability, electronic structure, magnetic properties and chemical bonding analysis of transition metal ammine borohydrides with amphoteric hydrogen for hydrogen storage**

S Kiruthika [a] and P Ravindran [a b c]

[a] Department of Physics, School of Basics and Applied Science, Central University of Tamil Nadu, Thiruvarur, India.

[b]Simulation Center for Atomic and Nanoscale MATerials (SCANMAT), Central University of Tamil Nadu, Thiruvarur, India

[c]Department of Chemistry, University of Oslo, Box 1033 Blindern, N0315, Norway.

Email Address: raviphy@cutn.ac.in

The optimized atomic positions at the equilibrium volume for $M(BH_4)_2(NH_3)_2$ $M$ = Sc, Ti, V, Cr, Fe, Co, Ni, and Cu obtained from the ground state crystal structure using spin-polarised optPBE-vdW functional.

| Compound Name and Space group | Atom Site and wyckoff position | x | y | z |
|---|---|---|---|---|
| $Sc(BH_4)_2(NH_3)_2$ | Sc 2a | 0.0000 | 0.0000 | 0.8928 |
| | B1 4c | 0.1671 | 0.2460 | 0.1919 |
| | H1 4c | 0.0054 | 0.2135 | 0.2596 |
| | H2 4c | 0.2239 | 0.4294 | 0.2181 |
| | H3 4c | 0.1431 | 0.2359 | 0.0486 |
| | H4 4c | 0.2963 | 0.1210 | 0.2350 |
| | N1 4c | 0.7231 | 0.1934 | 0.9780 |
| | H5 4c | 0.7637 | 0.3409 | 0.0171 |
| | H6 4c | 0.6028 | 0.2150 | 0.9040 |
| | H7 4c | 0.6699 | 0.1130 | 0.0740 |
| $Ti(BH_4)_2(NH_3)_2$ | Ti 2a | 0.0000 | 0.0000 | 0.8571 |
| | B1 4c | 0.2127 | 0.3194 | 0.1721 |
| | H1 4c | 0.0591 | 0.2458 | 0.2427 |
| | H2 4c | 0.2421 | 0.5067 | 0.2071 |
| | H3 4c | 0.1753 | 0.3087 | 0.0358 |
| | H4 4c | 0.3645 | 0.2163 | 0.2086 |
| | N1 4c | 0.7503 | 0.1362 | 0.9998 |
| | H5 4c | 0.7974 | 0.2703 | 0.0564 |
| | H6 4c | 0.6209 | 0.1798 | 0.9393 |
| | H7 4c | 0.7010 | 0.0318 | 0.0823 |
| $V(BH_4)_2(NH_3)_2$ | V 4c | 0.0000 | 0.2578 | 0.2500 |
| | B1 8d | 0.2443 | 0.0038 | 0.3435 |
| | N1 8d | 0.1743 | 0.2500 | 0.0983 |
| | H1 8d | 0.1113 | 0.5191 | 0.4076 |
| | H2 8d | 0.2181 | 0.4090 | 0.2691 |
| | H3 8d | 0.2356 | 0.1350 | 0.2965 |
| | H4 8d | 0.0796 | 0.9620 | 0.3856 |
| | H5 8d | 0.1435 | 0.1487 | 0.0543 |
| | H6 8d | 0.1438 | 0.3444 | 0.0543 |
| | H7 8d | 0.3352 | 0.2511 | 0.1118 |
| $Cr(BH_4)_2(NH_3)_2$ | Cr 4c | 0.0000 | 0.3439 | 0.2500 |

| | | | | |
|---|---|---|---|---|
| | B1 8d | 0.2603 | 0.9242 | 0.3775 |
| | N1 8d | 0.2111 | 0.3240 | 0.1254 |
| | H1 8d | 0.1304 | 0.5189 | 0.3322 |
| | H2 8d | 0.2007 | 0.2894 | 0.3483 |
| | H3 8d | 0.0881 | 0.9514 | 0.3524 |
| | H4 8d | 0.2921 | 0.9273 | 0.4749 |
| | H5 8d | 0.2135 | 0.2180 | 0.0894 |
| | H6 8d | 0.1826 | 0.3983 | 0.0622 |
| | H7 8d | 0.3570 | 0.3466 | 0.1488 |
| $Fe(BH_4)_2(NH_3)_2$ | H1 2a | 0.7391 | 0.3639 | 0.2022 |
| | H2 2a | 0.5520 | 0.4952 | 0.2454 |
| | H3 2a | 0.7557 | 0.4824 | 0.4103 |
| | H4 2a | 0.8848 | 0.0351 | 0.8712 |
| | H5 2a | 0.8862 | 0.2779 | 0.8692 |
| | H6 2a | 0.6902 | 0.1563 | 0.6831 |
| | H7 2a | 0.6527 | 0.1578 | 0.0027 |
| | H8 2a | 0.7431 | 0.9460 | 0.2086 |
| | H9 2a | 0.5509 | 0.8169 | 0.2407 |
| | H10 2a | 0.7496 | 0.8231 | 0.4124 |
| | H11 2a | 0.8225 | 0.5352 | 0.8435 |
| | H12 2a | 0.6331 | 0.6574 | 0.6512 |
| | H13 2a | 0.8230 | 0.7780 | 0.8451 |
| | H14 2a | 0.9535 | 0.6573 | 0.6116 |
| | B1 2a | 0.7747 | 0.1568 | 0.8578 |
| | B2 2a | 0.8086 | 0.6570 | 0.7335 |
| | N1 2a | 0.7127 | 0.4766 | 0.2529 |
| | N2 2a | 0.7119 | 0.8328 | 0.2540 |
| | Fe1 2a | 0.1267 | 0.1556 | 0.9166 |
| $Co(BH_4)_2(NH_3)_2$ | Co 8c | 0.1260 | 0.6396 | 0.9828 |
| | N1 8c | 0.0393 | 0.8021 | 0.9720 |
| | H18c | 0.0342 | 0.8554 | 0.0776 |
| | H2 8c | 0.0557 | 0.8793 | 0.8908 |
| | H3 8c | 0.9828 | 0.7648 | 0.9424 |
| | N2 8c | 0.2119 | 0.7755 | 0.0807 |
| | H4 8c | 0.1917 | 0.8280 | 0.1795 |
| | H5 8c | 0.2641 | 0.7218 | 0.1120 |
| | H6 8c | 0.2281 | 0.8562 | 0.0035 |
| | B1 8c | 0.1389 | 0.5557 | 0.7385 |
| | H7 8c | 0.1277 | 0.6419 | 0.6328 |
| | H8 8c | 0.1638 | 0.4381 | 0.6980 |
| | H9 8c | 0.0751 | 0.5404 | 0.8150 |
| | H10 8c | 0.1939 | 0.6033 | 0.8285 |
| | B2 8c | 0.1166 | 0.4635 | 0.1571 |
| | H11 8c | 0.1816 | 0.4903 | 0.0885 |
| | H12 8c | 0.1178 | 0.5122 | 0.2895 |
| | H13 8c | 0.1051 | 0.3333 | 0.1485 |
| | H14 8c | 0.0593 | 0.5222 | 0.0830 |
| $Ni(BH_4)_2(NH_3)_2$ | Ni 8c | 0.6263 | 0.0841 | 0.4795 |

| | | | | |
|---|---|---|---|---|
| | N1 8c | 0.5501 | 0.2508 | 0.4771 |
| | H1 8c | 0.5395 | 0.2936 | 0.5819 |
| | H2 8c | 0.5709 | 0.3320 | 0.4102 |
| | H3 8c | 0.4972 | 0.2209 | 0.4337 |
| | N2 8c | 0.7145 | 0.1986 | 0.5767 |
| | H4 8c | 0.6950 | 0.2682 | 0.6583 |
| | H5 8c | 0.7533 | 0.1318 | 0.6287 |
| | H6 8c | 0.7458 | 0.2586 | 0.5012 |
| | B1 8c | 0.6105 | 0.0366 | 0.2431 |
| | H7 8c | 0.6592 | 0.1231 | 0.3008 |
| | H8 8c | 0.5691 | 0.1041 | 0.1595 |
| | H9 8c | 0.5700 | 0.9848 | 0.3496 |
| | H10 8c | 0.6479 | 0.9429 | 0.1838 |
| | B2 8c | 0.6386 | 0.9206 | 0.6491 |
| | H11 8c | 0.6755 | 0.9225 | 0.5252 |
| | H12 | 0.6832 | 0.9429 | 0.7522 |
| | H13 | 0.6032 | 0.8094 | 0.6574 |
| | H14 | 0.5895 | 0.0215 | 0.6490 |
| $Cu(BH_4)_2(NH_3)_2$ | Cu 4c | 0.0000 | 0.1485 | 0.2500 |
| | B1 8d | 0.2336 | 0.0712 | 0.3751 |
| | N1 8d | 0.2048 | 0.1759 | 0.1282 |
| | H1 8d | 0.0909 | 0.5514 | 0.3496 |
| | H2 8d | 0.3703 | 0.4741 | 0.3311 |
| | H3 8d | 0.1917 | 0.2027 | 0.3443 |
| | H4 8d | 0.1989 | 0.0734 | 0.4739 |
| | H5 8d | 0.1722 | 0.1064 | 0.0629 |
| | H6 8d | 0.2045 | 0.2821 | 0.0966 |
| | H7 8d | 0.3510 | 0.1521 | 0.1523 |

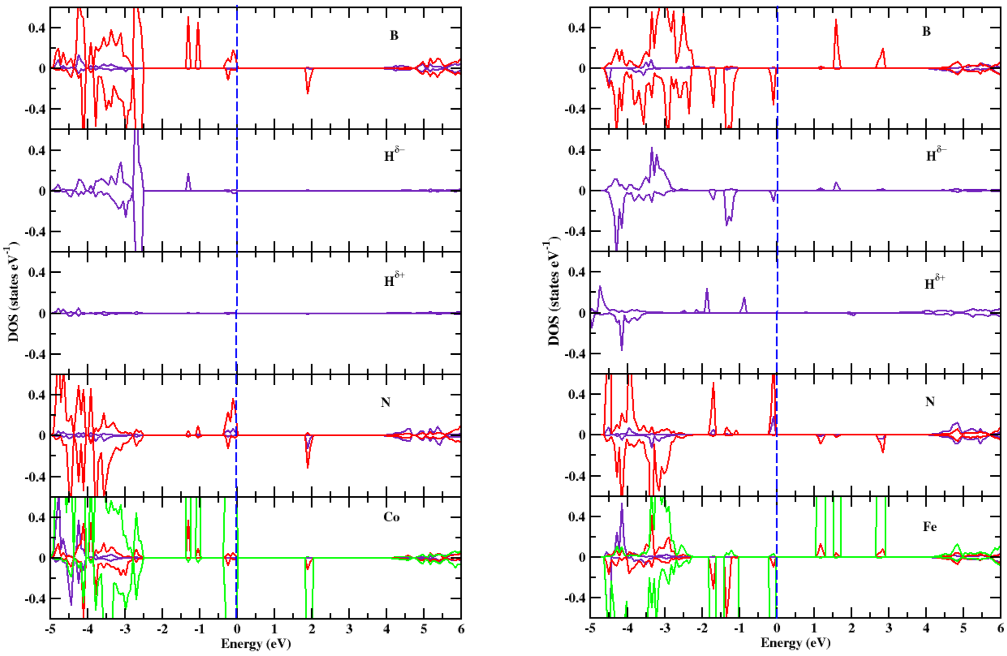


**Fig 1.** The partial density of states for $M(BH_4)_2(NH_3)_2$ where $M$ = Fe and Co obtained from optPBE-vdW functional at the equilibrium volume. The Fermi level is set to zero.

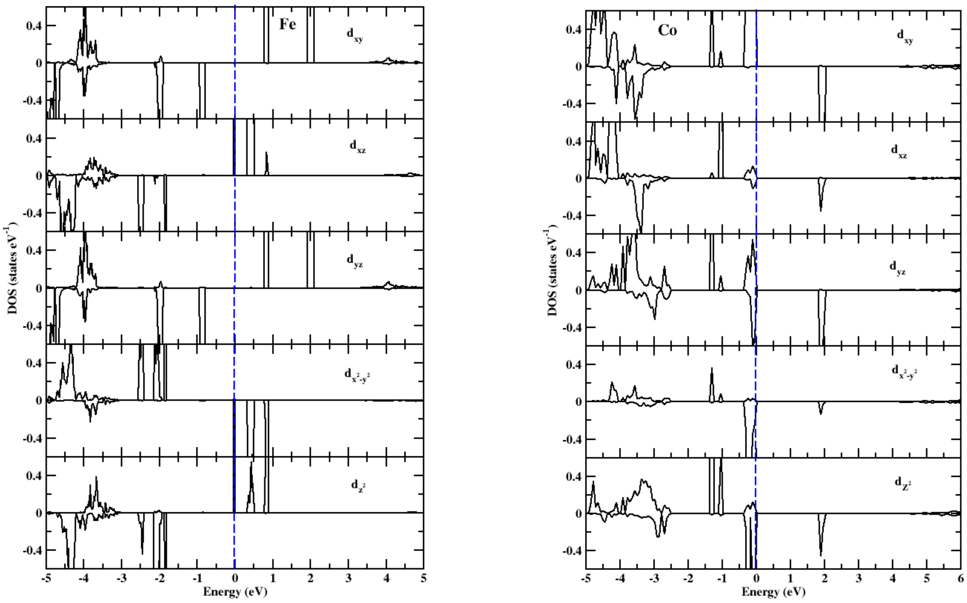


**Fig 2.** The orbital density of states for $M(BH_4)_2(NH_3)_2$ where $M$ = Fe and Co obtained from optPBE-vdW functional at the equilibrium volume. The Fermi level is set to zero.

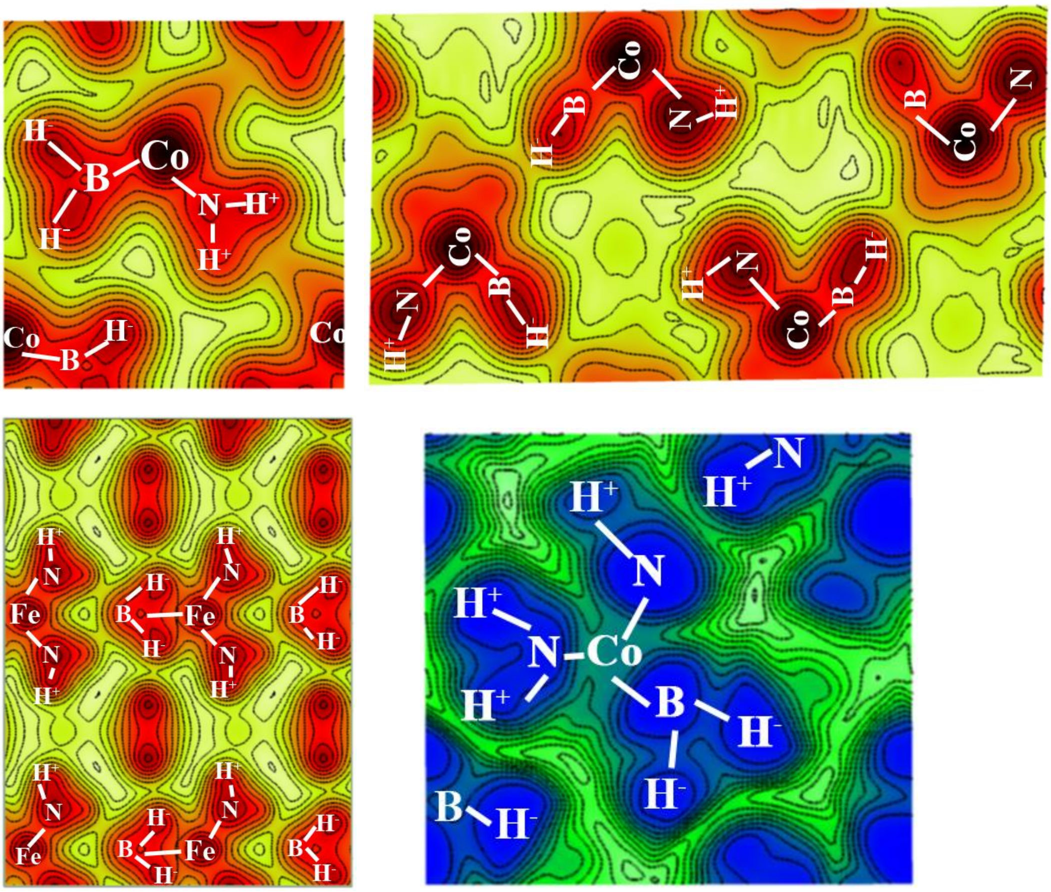


**Fig 3.** The Charge density and ELF plot for $M(BH_4)_2(NH_3)_2$ where $M$ = Fe and Co obtained from optPBE-vdW functional at the equilibrium volume. The Fermi level is set to zero.
